# Supplementary material for: A Versatile Software Systolic Execution Model for GPU Memory-Bound Kernels
Source: arXiv:1907.06154 source file (2019-09-06)
Supplement: Supplementary file 1 [file appendix.tex]

\appendix
\section*{Artifact Description Appendix:}\label{appendix}
A Versatile Software Systolic Execution Model for GPU Memory Bound Kernels

\subsection{Abstract}
This artifact contains the code for our SSAM-based applications for computing 2D-convolution, 2D/3D stencil. The same code can be used to reproduce the results in Fig.~\ref{fig:2d-conv-p100-v100},~\ref{fig:stencil-evaluation},~\ref{fig:stencil-temporal_blocking}.
The following sections give instructions for downloading, compiling, and executing the source code in order validate results.
%and parse the outputs also included in the artifact and explained below in detail.

\subsection{Description}
\subsubsection{Check-list (artifact meta information)}
\begin{itemize}
\item Algorithm:~
     \begin{itemize}
         \item \texttt{2D convolution}
	     \item \texttt{2D/3D stencil computation}
     \end{itemize}
\item Program:~
     \begin{itemize}
         \item \texttt{SSAM-based 2D convolution}
          \item \texttt{Arrayfire-based 2D convolution}
	     \item \texttt{cuFFT-based 2D convolution}
	     \item \texttt{cuDNN-based 2D convolution}
         \item \texttt{Halide-based 2D convolution}
	     \item \texttt{SSAM-based 2D/3D stencil computation}
	     \item \texttt{benchmark for 2D/3D stencil computation}
     \end{itemize}
\item {Compilation:} 
    \begin{itemize}
      \item \texttt{gcc} version 5.4 or above  
      \item \texttt{cmake} version 2.8 above
      \item \texttt{NVIDIA CUDA Toolkit} 10.0
         \begin{itemize}
         		\item \texttt{nvcc}
	            \item \texttt{NPP}
	            \item \texttt{cuFFT} 
         \end{itemize}
      \item \texttt{cuDNN} version 7.4
      \item \texttt{Arrayfire} 3.5 or above
      \item \texttt{Halide} release\_2017\_10\_30 or above
    \end{itemize}
\item Data set:~
	we generate random data for evaluation.
\item Hardware:
     \begin{itemize}
		  \item \texttt{PCIe-based NVIDIA Tesla P100 GPU}
	      \item \texttt{PCIe-based NVIDIA Tesla V100 GPU} 
     \end{itemize}
\item Output:~The shell scripts outputs the execution time for 2D convolution and 2D/3D stencil computation. In addition, the performance is also outputed for 2D/3D stencil in the unit of GCells/s.
\item Experiment workflow~
     \begin{itemize}
		  \item \texttt{Git clone source code}
	      \item \texttt{Build with cmake or Makefile}
          \item \texttt{Run script}
     \end{itemize}
\item Publicly available:~will be open source under MIT license
\end{itemize}
\label{subsubsec:check-list}

\subsubsection{How the software can be obtained}
\label{sec:how-to-obtain-software}
The implementations of SSAM-based algorithms will be open source.

\subsubsection{Hardware dependencies}
\begin{itemize}
\item Workstation with Nvidia P100/V100 GPU
  %\item {Run-time environment: }
  	\begin{itemize}
  	  \item Linux OS (tested on CentOS 7.4)
      \item NVIDIA GPU Driver v410.48 or above
      \item NVIDIA CUDA dirver 10.0
  	\end{itemize}
\end{itemize}
%%%%%%%%%%%%%%%%%%%%%%%%%%%%%%%%%%%%%%%%%%%%%%%%%%%%%%%%%%%%%%%%%%%%%
\subsection{Installation}
\begin{itemize}
\item git clone https://github.com/TBD RootDir
\item 2D convolution
  \begin{itemize}
    \item cd RootDir/conv2d\_SSAM
    \item make all
    \item run script evaluation.sh
    \item get result for 2D convolution
  \end{itemize}
\item 2D/3D stencil computation
\begin{itemize}
  \item cd RootDir/stencils
    \item make all
    \item run script evaluation.sh
    \item get result for 2D/3D convolution
  \end{itemize}
\end{itemize}  
\subsection{Notes}
Make sure the following options are set to
\begin{itemize}
    \item \texttt{nvcc} CUDA\_NVCC\_FLAGS
    	\begin{itemize}
    		\item For P100, -arch=sm\_60
            \item for V100, -arch=sm\_70
    	\end{itemize}
    \item \texttt{Halide} Halide\_Dir
    	\begin{itemize}
    		\item Set the Halide module path
    	\end{itemize}    
\end{itemize}
%For more details, please refer to README.md at the git repository.
